# Supplementary material for: Modeling Scale-free Graphs with Hyperbolic Geometry for Knowledge-aware Recommendation
Source: arXiv:2108.06468 source file (2022-01-02)
Supplement: Supplementary file 1 [file appendix.tex]

\section{Hyperbolic Related}

\subsection{Hyperbolic Model}
\subsubsection{Hyperbolic Space}

Let $\left<.,.\right>_\mathcal{M}$: $\mathbb{R}^{d+1} \times \mathbb{R}^{d+1} \rightarrow \mathbb{R}$ represent the Minkowski inner product, 
\begin{equation}
\left<\boldsymbol{x}, \boldsymbol{y} \right>_{\mathcal{M}} := -x_0y_0 + x_1y_1 + \dots + x_dy_d. 
\end{equation}   

The hyperbolic space is denoted by $\mathbb{H}^{d, K}$ in $d$ dimensions with constant negative \textbf{curvature} $-\frac{1}{K}$ where $K>0$, and the Euclidean tangent space centered at point $\boldsymbol{x} \in \mathbb{H}^{d, K}$ is denoted by $\mathcal{T}_{\boldsymbol{x}} \mathbb{H}^{d, K}$:

\begin{equation}
\begin{split}
& \mathbb{H}^{d, K} := \{\boldsymbol{x} \in \mathbb{R}^{d+1}: \left<\boldsymbol{x}, \boldsymbol{x}\right>_{\mathcal{M}} = -K, x_0 > 0\}; \\ 
& \mathcal{T}_{\boldsymbol{x}} \mathbb{H}^{d, K} := \{\boldsymbol{v} \in \mathbb{R}^{d+1}: \left<\boldsymbol{v}, \boldsymbol{x}\right>_{\mathcal{M}} = 0 \}.
 \end{split}
\end{equation} 

\subsubsection{Intrinsic Distance}
We use $||\boldsymbol{v}||_\mathcal{M} = \sqrt{\left<\boldsymbol{v}, \boldsymbol{v}\right>}_\mathcal{M}$ to denote the norm of $\boldsymbol{v} \in \mathcal{T}_{\boldsymbol{x}}\mathbb{H}^{d, K}$.  
The intrinsic distance between two points $\boldsymbol{x}, \boldsymbol{y}$ in $\mathbb{H}^{d, K}$ is defined as:
\begin{equation}
d_{\mathcal{M}}^K(\boldsymbol{x}, \boldsymbol{y}) = \sqrt{K} {\rm arcosh}(- \frac{\left<\boldsymbol{x}, \boldsymbol{y} \right>_{\mathcal{M}}}{K})
\end{equation} 

\subsubsection{Origin.} Let the point $\boldsymbol{o} = \{\sqrt{K}, 0, \dots, 0\} \in \mathbb{H}^{d, K}$ denote the north pole (orgin) in hyperbolic space $\mathbb{H}^{d, K}$, which will be used as a reference point to perform tangent space operations. For a point in $\boldsymbol{x'} \in \mathbb{R}^d$, we have $\left<(0, \boldsymbol{x'}), \boldsymbol{o}\right> = 0$. Thus, we can interpret $\boldsymbol{x} = (0, \boldsymbol{x'})$ as a point in $\mathcal{T}_{\boldsymbol{o}}\mathbb{H}^{d, K}$.

\subsubsection{Projections. } Projections to the hyperboloid manifold and its corresponding tangent space can be computed as follows, a point $\boldsymbol{x} = (x_0, \boldsymbol{x}_{1:d}) \in \mathbb{R}^{d+1}$ can be projected to hyperbolic manifold $\mathbb{H}^{d, K}$: 
\begin{equation}
{\rm Prj}_{\mathbb{R}^{d+1} \rightarrow \mathbb{H}^{d,K} } (\boldsymbol{x}) := (\sqrt{K + ||\boldsymbol{x}_{1:d}||_2^2}, \boldsymbol{x}_{1:d}) 
\end{equation} 

Similarly, for a point $\boldsymbol{v}\in \mathbb{R}^d$, we can project it to tangent space $\mathcal{T}_{\boldsymbol{o}} \mathbb{H}^{d, K}$:
\begin{equation}
\label{eq:project_tangent}
{\rm Prj}_{\mathbb{R}^{d+1} \rightarrow \mathcal{T}_{{\boldsymbol x}}\mathbb{H}^{d,K}} (\boldsymbol{v}) :=  \boldsymbol{v} + \left<\boldsymbol{x}, \boldsymbol{v} \right>_{\mathcal{M}}\boldsymbol{x}
\end{equation}

If the $\boldsymbol{x} = \boldsymbol{o}$, Equation~\ref{eq:project_tangent} can be simplified as:
\begin{equation}
\label{eq:project_tangent}
{\rm Prj}_{\mathbb{R}^{d+1} \rightarrow \mathcal{T}_{{\boldsymbol o}}\mathbb{H}^{d,K}} (\boldsymbol{v}) :=  \boldsymbol{v} + \left<\boldsymbol{o}, \boldsymbol{v} \right>_{\mathcal{M}}\boldsymbol{o} = (0, \boldsymbol{v}_{1:d})
\end{equation}

\subsubsection{Mapping between Tangent Space and Hyperbolic Space.}
\begin{proposition}
For $\boldsymbol{x} \in \mathbb{H}^{d, K}$, $\boldsymbol{v} \in \mathcal{T}_{\boldsymbol{x}}\mathbb{H}^{d, K}$ and $\boldsymbol{y} \in \mathbb{H}^{d, K}$ such that $\boldsymbol{v} \neq \boldsymbol{0}$ and $\boldsymbol{y} \neq \boldsymbol{x}$, the exponential and logarithmic maps of the hyperboloid model are given by:
\begin{equation}
\begin{split}
& \begin{matrix}\prod\end{matrix}^{{\rm exp}, K}_{\boldsymbol{x}}(\boldsymbol{v}) = cosh(\frac{|| \boldsymbol{v}||_{\mathcal{M}}}{\sqrt{K}})\boldsymbol{x} + \sqrt{K}sinh(\frac{||\boldsymbol{v}||_\mathcal{M}}{\sqrt{K}})\frac{\boldsymbol{v}}{||\boldsymbol{v}||_{\mathcal{M}}}; \\
& \begin{matrix}\prod\end{matrix}^{{\rm log}, K}_{\boldsymbol{x}}(\boldsymbol{y}) = d^K_{\mathcal{M}} (\boldsymbol{x}, \boldsymbol{y}) \frac{\boldsymbol{y} + \frac{1}{K} \left<\boldsymbol{x}, \boldsymbol{y}\right>_{\mathcal{M}} \boldsymbol{x}}{|| \boldsymbol{y} + \frac{1}{K} \left<\boldsymbol{x}, \boldsymbol{y}\right>_{\mathcal{M}} \boldsymbol{x} ||_{\mathcal{M}}} 
\end{split}
\end{equation}
\end{proposition}

If $\boldsymbol{x} = \boldsymbol{o}$, the above mapping can be rewritten as:
\begin{equation}
\begin{split}
& \begin{matrix}\prod\end{matrix}^{{\rm exp}, K}_{\boldsymbol{o}}(\boldsymbol{v}) = (\sqrt{K} cosh(|| \boldsymbol{v_{1:d}}||_2), \sqrt{K} sinh(\frac {|| \boldsymbol{v_{1:d}}||_2}{\sqrt{K}} ) \frac{\boldsymbol{v_{1:d}}}{|| \boldsymbol{v_{1:d}}||_2}); \\
& \begin{matrix}\prod\end{matrix}^{{\rm log}, K}_{\boldsymbol{o}}(\boldsymbol{y}) = (0, \sqrt{K} arcosh(\frac{y_0}{\sqrt{K}})\frac{ \boldsymbol{y_{1:d}}}{ || \boldsymbol{y_{1:d}} ||_2}) 
\end{split}
\end{equation}

\subsection{Hyperboloid Manifold}

\subsubsection{Hyperboloid Space and Intrinsic Distance}
In hyperboloid manifold, the curvature $-\frac{1}{K}=-1$, we use $\mathbb{H}^{d, 1}$ to denote the hyperboloid manifold and $\mathcal{T}_{\boldsymbol{x}}\mathbb{H}^{d, 1}$ to denote the tangent space point at $\boldsymbol{x} \in \mathbb{H}^{d, 1}$: 

\begin{equation}
\begin{split}
& \mathbb{H}^{d, 1} := \{\boldsymbol{x} \in \mathbb{R}^{d+1}: \left<\boldsymbol{x}, \boldsymbol{x}\right>_{\mathcal{M}} = -1, x_0 > 0\} \\
& \mathcal{T}_{\boldsymbol{x}} \mathbb{H}^{d, 1} := \{\boldsymbol{v} \in \mathbb{R}^{d+1}: \left<\boldsymbol{v}, \boldsymbol{x}\right>_{\mathcal{M}} = 0 \}
\end{split}
\end{equation}

The intrinsic distance of hyperboloid manifold between two points $\boldsymbol{x}, \boldsymbol{y}$ in $\mathbb{H}^{d, 1}$ is:
\begin{equation}
d_{\mathcal{M}}(\boldsymbol{x}, \boldsymbol{y}) = {\rm arcosh}(-\left<\boldsymbol{x}, \boldsymbol{y} \right>_{\mathcal{M}})
\end{equation} 

\subsubsection{Projections}
The projection in hyperboloid manifold $\mathbb{H}^{d, 1}$ can be simplified as:
\begin{equation} 
\begin{split}
& {\rm Prj}_{\mathbb{R}^{d+1} \rightarrow \mathbb{H}^{d,1} } (\boldsymbol{x}) := (\sqrt{1 + ||\boldsymbol{x}_{1:d}||_2^2}, \boldsymbol{x}_{1:d}); \\
& {\rm Prj}_{\mathbb{R}^{d+1} \rightarrow \mathcal{T}_{{\boldsymbol x}}\mathbb{H}^{d,1}} (\boldsymbol{v}) :=  (o, \boldsymbol{v}_{1:d}).
\end{split}
\end{equation}

\subsubsection{Mapping between Tangent Space and Hyperboloid Manifold.}

\begin{proposition}
For $\boldsymbol{x} \in \mathbb{H}^{d, 1}$, $\boldsymbol{v} \in \mathcal{T}_{\boldsymbol{x}}\mathbb{H}^{d, 1}$ and $\boldsymbol{y} \in \mathbb{H}^{d,1}$ such that $\boldsymbol{v} \neq \boldsymbol{0}$ and $\boldsymbol{y} \neq \boldsymbol{x}$, the exponential and logarithmic maps of the hyperboloid model are given by:
\begin{equation}
\begin{split}
& \begin{matrix}\prod\end{matrix}^{\rm exp}_{\boldsymbol{x}}(\boldsymbol{v}) = cosh(|| \boldsymbol{v}||_{\mathcal{M}})\boldsymbol{x} + sinh(||\boldsymbol{v}||_\mathcal{M})\frac{\boldsymbol{v}}{||\boldsymbol{v}||_{\mathcal{M}}}; \\
& \begin{matrix}\prod\end{matrix}^{\rm log}_{\boldsymbol{x}}(\boldsymbol{y}) = d^1_{\mathcal{M}} (\boldsymbol{x}, \boldsymbol{y}) \frac{\boldsymbol{y} +  \left<\boldsymbol{x}, \boldsymbol{y}\right>_{\mathcal{M}} \boldsymbol{x}}{|| \boldsymbol{y} + \left<\boldsymbol{x}, \boldsymbol{y}\right>_{\mathcal{M}} \boldsymbol{x} ||_{\mathcal{M}}} 
\end{split}
\end{equation}
\end{proposition}

Similarly, when the $\boldsymbol{x} = \boldsymbol{o}$, we have: 
\begin{equation}
\begin{split}
& \begin{matrix}\prod\end{matrix}^{\rm exp}_{\boldsymbol{o}}(\boldsymbol{v}) = (cosh(|| \boldsymbol{v_{1:d}}||_2), sinh(|| \boldsymbol{v_{1:d}}||_2 ) \frac{\boldsymbol{v_{1:d}}}{|| \boldsymbol{v_{1:d}}||_2}); \\
& \begin{matrix}\prod\end{matrix}^{\rm log}_{\boldsymbol{o}}(\boldsymbol{y}) = (0, arcosh(y_0)\frac{ \boldsymbol{y_{1:d}}}{ || \boldsymbol{y_{1:d}} ||_2}) 
\end{split}
\end{equation}
